# Supplementary material for: Hierarchical Policy Blending as Inference for Reactive Robot Control
Source: arXiv:2210.07890 source file (2024-07-29)
Supplement: Supplementary file 1 [file appendix.tex]

\clearpage
\onecolumn
\appendix
\subsection{Weighted Product of multivariate Gaussian distributions}
\label{app:PoG}
Lets consider the Gaussian case 
\begin{align*}
    p(\hat{\beta}\mid x) &= \frac{p(x\mid\hat{\beta})p(\beta)}{p(x)}\\
    &\propto p(x\mid\hat{\beta})p(\beta)\\
    &=\exp\left(\hat\beta^{T}\mathbb{E}(x) - \log A(\hat\beta)\right),
\end{align*}
where each individual expert is represented as $E_{i}(x) = -\log\mathcal{N}\left(x\mid\mu_{i},\Lambda_{i}^{-1}\right)$. In this case the quantity $x$ expresses some arbitrary random variable, e.g. the action in case of a policy.
After some derivations, it follows 
\begin{align}
    \label{eq:appendix:exponential_family}
    p(\hat{\beta}\mid x) &\propto \exp
    \begin{aligned}[t]
        &\left(\xi(\hat{\beta}) + \eta^{T}(\hat{\beta}) x \right.\\
        &\left.- \frac{1}{2} x^{T}\Lambda(\hat{\beta}) x - \log A(\hat\beta)\right),
    \end{aligned}
\end{align}
with 
\begin{align*}
    A(\hat\beta) &= \int_{x}\exp\left(\xi(\hat{\beta}) + \eta^{T}(\hat{\beta}) x - \frac{1}{2} x^{T}\Lambda(\hat{\beta}) x\right)dx \\
    \xi(\hat{\beta}) &= \sum_{i=1}^{N} -\frac{d \beta_{i}}{2}\log(2\pi) + \frac{\beta_{i}}{2}\log\left| \Lambda_{i}\right| - \frac{\beta_{i}}{2} \mu_{i}^{T}\Lambda\mu_{i}\\
    \eta(\hat{\beta}) &= \sum_{i=1}^{N}\beta_{i}\Lambda_{i}\mu_{i}\\
    \Lambda(\hat{\beta}) &= \sum_{i=1}^{N}\beta_{i}\Lambda_{i}.
\end{align*}
Due to the quadratic nature of a Gaussian distribution we see that $A(\hat\beta)$ is a Gaussian integral of the form 
\begin{align*}
    A(\hat\beta) &=\exp\left(\xi)\right)\int_{x}\exp\left(\xi\eta^{T} x - \frac{1}{2} x^{T}\Lambda x\right)dx,
\end{align*}
where we we omitted $\hat\beta$ in terms of conciseness. It is straightforward to see that after integration by substitution we result in 
\begin{align*}
    A(\hat\beta) &=\exp\left(\xi  + \frac{1}{2}\eta^{T}\Lambda^{-1}\eta)\right)\int\exp\left(- \frac{1}{2} z^{T}\Lambda z\right)dz,
\end{align*}
with $z = x - \Lambda^{-1}\eta$ resulting in a closed form solution 
\begin{align}
    \label{eq:appendix:gaussian_integral_solution}
    A(\hat\beta) &= \frac{(2\pi)^{d/2}}{\left|\Lambda\right|^{1/2}}\exp\left(\xi + \frac{1}{2}\eta^{T}\Lambda^{-1}\eta\right).
\end{align}
Plug Equation \ref{eq:appendix:gaussian_integral_solution} back into Equation \ref{eq:appendix:exponential_family} results in
\begin{align*}
    p(\hat{\beta}\mid x) &\propto (2\pi)^{-d/2}\left|\Lambda\right|^{1/2} \\
    &\exp\left(-\frac{1}{2}x^{T}\Lambda x + \eta^{T} x - \frac{1}{2} \eta^{T} \Lambda^{-1} \eta\right),
\end{align*}
where we omitted the dependency on $\hat\beta$.
Utilizing \textit{completing the squares} gives the final results 
\begin{align*}
    \mathcal{N}\left(x\middle|\Lambda^{-1}\eta, \Lambda^{-1}\right).
\end{align*}
This results shows exactly what we were looking for. A product of a Gaussian distribution produces a Gaussian distribution with the influence of each component weighted by the temperature parameters $\hat\beta$.
\subsection{Probabilistic inference for policy blending}

To infer the optimal weights $\beta_0, \cdots \beta_{\nexperts}$, we formalize the optimization problem as an inference problem.

We propose a hierarchical method \ref{sec:approach:pseudocode} that blends reactive policy utilizing a probabilistic inference formulation. Infering $\beta^{*}$ idea:
\begin{enumerate}
    \item 
    $p(\beta \mid \mathcal{O}_{\tau}, \vec{s}_{1}) \propto p(\mathcal{O}_{\tau} \mid \beta , \vec{s}_{1}) p(\beta \mid  \vec{s}_{1})$
    \item 
    $q^{*}(\beta) = \argmin_{q(\beta)} \KL{q(\beta)}{p(\beta \mid \mathcal{O}_{\tau}, \vec{s}_{1})}$
    \item 
    $\beta^{*} = \E{q^{*}(\beta)}$
\end{enumerate}
Closer look on 1.) states the Bayes rule
\begin{align}
    p(\beta \mid \mathcal{O}_{\tau}, s_{1} ; \theta) \propto &
    p(\mathcal{O}_{\tau} \mid \beta , s_{1}) p(\beta \mid  s_{1}),
\end{align}
with posterior is the product of likelihood and prior. The likelihood is a marginalization over the trajectories
\begin{align}
    p(\mathcal{O}_{\tau} \mid \beta , s_{1}) =
    & \int p(\mathcal{O}_{\tau}, \tau\mid \beta , s_{1}) \,d\tau\\
    =& \int p(\mathcal{O}_{\tau}\mid \tau, s_{1}) p(\tau\mid \beta , s_{1}) \,d\tau\\
    =& \iint p(\mathcal{O}_{\mat{A}, \mat{S}}\mid \mat{A}, \mat{S}, s_{1}) p(\mat{A}, \mat{S}\mid \beta , s_{1}) \,d\mat{A}\,d\mat{S},
\end{align}
with trajectory $\tau = \{\mat{A}, \mat{S}\}$, concatenated action vector $\mat{A} = [\vec{a}_{1}, \cdots]$ and state matrix  $\mat{S} = [\vec{s}_{2}, \cdots]$. The conditional distribution for optimality 
\begin{align}
    p(\mathcal{O}_{\mat{A}, \mat{S}}\mid \mat{A}, \mat{S}, s_{1}) =& \prod_{t=1}^{H} p(\mathcal{O}_{t}=1\mid, \vec{a}_{t}, \vec{s}_{t})
\end{align}
and the trajectory distribution 
\begin{align}
    p(\mat{A}, \mat{S}\mid \beta , s_{1}) =& \prod_{t=1}^{H} p(\vec{s}_{t+1}\mid, \vec{a}_{t}, \vec{s}_{t})p(\vec{a}_{t}\mid \beta, \vec{s}_{t}).
\end{align}
The conditional probability $p(\vec{a}_{t}\mid \beta,  \vec{s}_{t})$ doesn't represent a policy. The quantity has to consider the optimality as well. Hence, $p(\vec{a}_{t}\mid \beta, \vec{s}_{t})$ corresponds to a prior distribution. Since we don't want to bias the model, we take the prior as uninformative as possible. Thus, we set it equal for each action. In other words, we do not restrict the model to favor one action in a state. \\
Lets have a closer look on 2.) where we approximate the posterior distribution 
\begin{align}
    q^{*}(\beta) = \argmin_{q(\beta)}\quad \KL{q(\beta)}{p(\beta \mid \mathcal{O}_{\tau}, \vec{s}_{1})},
\end{align}
minimizing the KL divergence. Since we consider a sequence of temperatures, we consider $q(\beta) = \prod_{t=1}^{H}q^{H}(\beta)$. Following the KL-Divergence, we get
\begin{align}
    \KL{q(\beta)}{p(\beta \mid \mathcal{O}_{\tau}, \vec{s}_{1})} &= 
    \begin{aligned}[t]
        & \H[q(\beta)]{p(\beta \mid \mathcal{O}_{\tau}, \vec{s}_{1})} \\
        &- \H[]{q(\beta)},
    \end{aligned}
\end{align}
the Cross-Entropy subtracted by the Shannon Entropy. The Shannon Entropy $\H[]{q(\beta)}$ ensures that the approximation of the posterior distribution stays as random as possible. In other words, $\H[]{q(\beta)}$ mitigates the effect of collapsing in the parameter space of $\beta$. The Cross-Entropy is 
\begin{align}
    \H[q(\beta)]{
    p(\beta \mid \mathcal{O}_{\tau}, \vec{s}_{1})
    } 
    \propto & 
    \H[q(\beta)]{
        p(\mathcal{O}_{\tau} \mid \beta , \vec{s}_{1}) p(\beta \mid  \vec{s}_{1})
        } \\
    = & 
    \begin{aligned}[t]
    &\H[q(\beta)]{
        p(\mathcal{O}_{\tau} \mid \beta , \vec{s}_{1})}\\
    &+     
    \H[q(\beta)]{p(\beta \mid  \vec{s}_{1})
        },
    \end{aligned}
\end{align}
with the former and the latter quantity on the right hand side corresponding to the cross-entropy to the likelihood and the prior distribution, respectively. Hence, minimizing the KL-divergence tries to minimize the distance to the prior as well as to the likelihood. The first cross-entropy corresponds to 
\begin{align}
    \H[q(\beta)]{
    p(\mathcal{O}_{\tau} \mid \beta , \vec{s}_{1})
    } 
    \propto & 
    \begin{aligned}[t]
    \int &q(\beta) 
        \log\biggl[\iint \prod_{t=1}^{H} p(\mathcal{O}_{t}=1\mid, \vec{a}_{t}, \vec{s}_{t}) \\
        & p(\vec{s}_{t+1}\mid, \vec{a}_{t}, \vec{s}_{t}) \,d\mat{A}\,d\mat{S}
        \biggr]\, d\beta.
    \end{aligned}
\end{align}
The quantity looks intractable (if no closed-form is available) because of the integral within the logarithm. Hence, we make use of variational inference introducing a variational distribution 
\begin{align}
    q(\tau) = q(\vec{s}_{0})\prod_{t=1}^{H}q(\vec{s}_{t+1}\mid, \vec{a}_{t}, \vec{s}_{t})\pi(\vec{a}_{t}\mid \beta_{t}, \vec{s}_{t}).
\end{align}
This auxilary distribution factorizes to the product of inital distribution, the dynamics, and the policy. As our variational distribution can't modify the initial distribution and the dynamics, we assume that
\begin{align}
    q(\vec{s}_{0}) =& p(\vec{s}_{0})\\
    q(\vec{s}_{t+1}\mid, \vec{a}_{t}, \vec{s}_{t}) =& p(\vec{s}_{t+1}\mid, \vec{a}_{t}, \vec{s}_{t}).
\end{align}
Additionally, the policy is given as product of experts
\begin{align}
    \pi(\vec{a}_{t}\mid \beta_{t}, \vec{s}_{t}) &= 
    \frac{1}{Z(\beta)}\prod_{n=1}^{N}\pi_{n}(\vec{a}, \vec{s})^{\beta_{n}}\\
    &= c(\vec{a}_{t})\exp\left(\beta^{T} E(\vec{a}_{t}, \vec{s}_{t}) + \log A(\beta)\right)\\
    &= \mathcal{N}\left(x\middle|\Lambda^{-1}\eta, \Lambda^{-1}\right),
\end{align}
which takes a form of a Gaussian if all policies are Gaussian. Hence, $\eta(\hat{\beta}) = \sum_{i=1}^{N}\beta_{i}\Lambda_{i}\mu_{i}$ and $\Lambda(\hat{\beta}) = \sum_{i=1}^{N}\beta_{i}\Lambda_{i}$. The Cross-Entropy terms reduces to 
\begin{align}
    \H[q(\beta)]{
    p(\mathcal{O}_{\tau} \mid \beta , \vec{s}_{1})
    } \propto  & \\
    \int q(\beta) &\E[\tau\sim q(\tau\mid\beta)]{\log\biggl[\prod_{t=1}^{H}\frac{ p(\mathcal{O}_{t}=1\mid, \vec{a}_{t}, \vec{s}_{t})}{\pi(\vec{a}_{t}\mid \beta_{t}, \vec{s}_{t})} \biggr]}\,d\beta.
\end{align}
\subsection{Parametric Bayesian MPC}
Considering a parameterized distribution $q(\beta ; \theta)$ the objective becomes
\begin{align}
    J(\theta) &= \min_{\theta} \quad\KL{q(\beta; \theta)}{p(\beta \mid \mathcal{O}_{\tau}, \vec{s}_{1})}, \\
    &= \max_{\theta} \quad -\KL{q(\beta; \theta)}{p(\beta \mid \mathcal{O}_{\tau}, \vec{s}_{1})}, \\
    &\propto \min_{\theta}\quad 
    \begin{aligned}[t]
    \biggl[
    & \H[q(\beta; \theta)]{q(\beta; \theta)}\\
    & - \H[q(\beta; \theta)]{
    p(\mathcal{O}_{\tau} \mid \beta , \vec{s}_{1})
    } \\
    & - \H[q(\beta; \theta)]{p(\beta \mid  \vec{s}_{1})}
    \biggr].
    \end{aligned}
\end{align}
To get the gradient, we apply the score-function trick / log-ratio trick / REINFORCE 
\begin{align}
    \nabla_{\theta}J(\theta) &= 
    \begin{aligned}[t]
    & + \E[q(\beta; \theta)]{\nabla_{\theta}\log q(\beta; \theta)
    \log p(\mathcal{O}_{\tau} \mid \beta , \vec{s}_{1})
    } \\
    & + \E[q(\beta; \theta)]{\nabla_{\theta}\log q(\beta; \theta)
    \log p(\beta \mid  \vec{s}_{1})}\\
    & - \E[q(\beta; \theta)]{\nabla_{\theta}\log q(\beta; \theta)
    \log q(\beta)}. 
    \end{aligned} \\
    & \approx \frac{1}{S}\sum_{s=1}^{S} \nabla_{\theta}\log q(\beta; \theta) \biggl[\log \frac{p(\mathcal{O}_{\tau} \mid \beta , \vec{s}_{1})p(\beta \mid  \vec{s}_{1})}{q(\beta)} \biggr],
\end{align}
which represents a weighting of the gradients. To optimize the parameters of a parameterized distribution, it is necessary to consider the strucure of the parameter space. Hence, we utilize mirror descent a trust region optimization algorithm 
\begin{align}
    \argmax_{\Delta\theta} \nabla_{\theta}J(\theta)^{T} \Delta\theta + \eta \KL{p(\beta ; \theta)}{p(\beta ; \theta + \Delta\theta)}\\\\
    \argmax_{\Delta\theta}\quad J(\theta + \Delta\theta) \approx J(\theta) + \nabla_{\theta} J(\theta)^{T} \Delta\theta\\
    \textrm{s.t.}\quad \KL{p(\beta ; \theta)}{p(\beta ; \theta + \Delta\theta)} \leq \epsilon \approx \frac{1}{2}\Delta\theta^{T}\mathrm{F}\Delta\theta
\end{align}
Mirror descent seeks for an optimal policy in a trust-region around the current parameter. The objective is approximate by the first order Taylor-expansion. A second order Taylor-expansion approximates the KL divergence. The optimization step should end up in 
\begin{align}
    \theta_{k+1} = \theta_{k} + \eta^{-1}\mathrm{F}^{-1}\nabla_{\theta} J(\theta).
\end{align}
If we consider a Lagrang optimization procedure with a KL-divergence constraining the policy change, we end up with a learning rate $\eta^{-1} = \sqrt{\epsilon / (\nabla_{\theta}^{T}J(\theta)\mathrm{F}^{-1}\nabla_{\theta}J(\theta))}$. However, similar to TRPO, if we use the automatic learning rate adjustment, we normally use a learning rate still
\begin{align}
    \theta_{k+1} = \theta_{k} - \alpha \sqrt{\frac{\epsilon}{ (\nabla_{\theta}^{T}J(\theta)\mathrm{F}^{-1}\nabla_{\theta}J(\theta))}}\mathrm{F}^{-1}\nabla_{\theta} J(\theta).
\end{align}
Due to the approximation, the additional learning rate $\alpha$ stabilizes the learning process. 

We only take one step of the gradient update and afterwards use the approximated / updated posterior distribution as new prior. Following these procedure, we use an appropriate FIM at each step.

\begin{align*}
    \dot{\boldsymbol{q}}_{\textrm{D}} = J^{\dagger}\dot{\boldsymbol{x}}_{\textrm{VR}} + (\boldsymbol{I} - J^{\dagger^\textrm{T}}J^{\dagger})\nabla g(\boldsymbol{q}_\textrm{R})
\end{align*}
